# Supplementary material for: Evolution of induced earthquakes from dimensionless scaling
Source: arXiv:1410.6633 ancillary file (2014-10-24)
Supplement: Supplementary file 1 [file USGS_input.pdf]

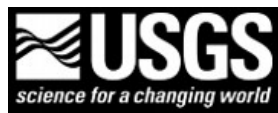**Earthquake Hazards Program****Earthquake Archive Search & URL Builder**

Search results are limited to 20,000 events.

- [Help](#)
- [About ANSS Comprehensive Catalog](#)

**Basic Search Options****DATE & TIME**

Start (UTC)  End (UTC)

**MAGNITUDE**

Minimum  Maximum

**GEOGRAPHIC REGION**

Currently searching custom region

[Clear Region](#)**Rectangle**

Decimal degree coordinates. North must be greater than South.  
East must be greater than West.

North   
West  East   
South

**Circle**

Center Latitude   
Center Longitude   
Inside Radius (km)   
Outside Radius (km)

**Advanced Search Options****DEPTH (KM)**

Minimum  Maximum

**AZIMUTHAL GAP**

Minimum  Maximum

**REVIEW STATUS**

- ☒ Any  
☐ Automatic  
☐ Reviewed

**+ EVENT TYPE****+ IMPACT** (PAGER, SHAKEMAP, DYFI)**+ CATALOG****+ CONTRIBUTOR****- PRODUCT TYPE**

- ☒ Any ☐ Associate  
☐ CAP ☐ Disassociate  
☐ DYFI? ☐ Eq-location-map  
☐ Finite Fault ☐ Focal Mechanism  
☐ General Link ☐ General-text  
☐ GeoServe ☐ Historical-moment-tensor-map  
☐ Historical-seismicity-map ☐ Image  
☐ Impact Text ☐ Impact Link  
☐ LossPAGER  
☐ Moment Tensor ☐ Moreinformation  
☐ Nearby Cities ☐ Origin  
☐ P-Wave Travel Times ☐ Phase Data

**Output Options****FORMAT**

- ☐ Map & List  
☒ CSV  
☐ KML  
☐ QuakeML  
☐ GeoJSON

**ORDER BY**

- ☒ Time - Newest First  
☐ Time - Oldest First  
☐ Magnitude - Largest First  
☐ Magnitude - Smallest First

**LIMIT RESULTS**

Number of Events  Offset

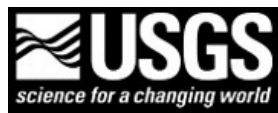**Earthquake Hazards Program****Earthquake Archive Search & URL Builder**

Search results are limited to 20,000 events.

- [Help](#)
- [About ANSS Comprehensive Catalog](#)

**Basic Search Options****DATE & TIME**

Start (UTC) End (UTC)

**MAGNITUDE**

Minimum Maximum

**GEOGRAPHIC REGION**

Currently searching custom region

[Clear Region](#)**Rectangle**

Decimal degree coordinates. North must be greater than South.  
East must be greater than West.

North  
  
West East  
   
South

**Circle**

Center Latitude Center Longitude  
   
Inside Radius (km) Outside Radius (km)

**Advanced Search Options****DEPTH (KM)**

Minimum Maximum

**AZIMUTHAL GAP**

Minimum Maximum

**REVIEW STATUS**

- ☒ Any  
☐ Automatic  
☐ Reviewed

**+ EVENT TYPE****+ IMPACT** (PAGER, SHAKEMAP, DYFI)**+ CATALOG****+ CONTRIBUTOR****- PRODUCT TYPE**

- ☒ Any ☐ Associate  
☐ CAP ☐ Disassociate  
☐ DYFI? ☐ Eq-location-map  
☐ Finite Fault ☐ Focal Mechanism  
☐ General Link ☐ General-text  
☐ GeoServe ☐ Historical-moment-tensor-map  
☐ Historical-seismicity-map ☐ Image  
☐ Impact Text ☐ Impact Link  
☐ LossPAGER  
☐ Moment Tensor ☐ Moreinformation  
☐ Nearby Cities ☐ Origin  
☐ P-Wave Travel Times ☐ Phase Data

**Output Options****FORMAT**

- ☐ Map & List  
☒ CSV  
☐ KML  
☐ QuakeML  
☐ GeoJSON

**ORDER BY**

- ☒ Time - Newest First  
☐ Time - Oldest First  
☐ Magnitude - Largest First  
☐ Magnitude - Smallest First

**LIMIT RESULTS**

Number of Events Offset

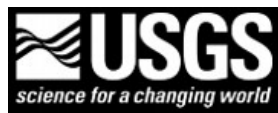**Earthquake Hazards Program****Earthquake Archive Search & URL Builder**

Search results are limited to 20,000 events.

- [Help](#)
- [About ANSS Comprehensive Catalog](#)

**Basic Search Options****DATE & TIME**

Start (UTC) End (UTC)

**MAGNITUDE**

Minimum Maximum

**GEOGRAPHIC REGION**

Currently searching custom region

[Clear Region](#)**Rectangle**

Decimal degree coordinates. North must be greater than South.  
East must be greater than West.

North  
  
West East  
   
South

**Circle**

Center Latitude Center Longitude  
   
Inside Radius (km) Outside Radius (km)

**Advanced Search Options****DEPTH (KM)**

Minimum Maximum

**AZIMUTHAL GAP**

Minimum Maximum

**REVIEW STATUS**

- ☒ Any  
☐ Automatic  
☐ Reviewed

**+ EVENT TYPE****+ IMPACT** (PAGER, SHAKEMAP, DYFI)**+ CATALOG****+ CONTRIBUTOR****- PRODUCT TYPE**

- ☒ Any ☐ Associate  
☐ CAP ☐ Disassociate  
☐ DYFI? ☐ Eq-location-map  
☐ Finite Fault ☐ Focal Mechanism  
☐ General Link ☐ General-text  
☐ GeoServe ☐ Historical-moment-tensor-map  
☐ Historical-seismicity-map ☐ Image  
☐ Impact Text ☐ Impact Link  
☐ LossPAGER  
☐ Moment Tensor ☐ Moreinformation  
☐ Nearby Cities ☐ Origin  
☐ P-Wave Travel Times ☐ Phase Data

**Output Options****FORMAT**

- ☐ Map & List  
☒ CSV  
☐ KML  
☐ QuakeML  
☐ GeoJSON

**ORDER BY**

- ☒ Time - Newest First  
☐ Time - Oldest First  
☐ Magnitude - Largest First  
☐ Magnitude - Smallest First

**LIMIT RESULTS**

Number of Events Offset

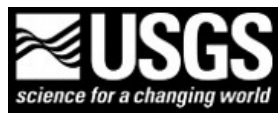**Earthquake Hazards Program****Earthquake Archive Search & URL Builder**

Search results are limited to 20,000 events.

- [Help](#)
- [About ANSS Comprehensive Catalog](#)

**Basic Search Options****DATE & TIME**

Start (UTC)

End (UTC)

**MAGNITUDE**

Minimum

Maximum

**GEOGRAPHIC REGION**

Currently searching custom region

[Clear Region](#)**Rectangle**

Decimal degree coordinates. North must be greater than South.

East must be greater than West.

|                                   |                                  |
|-----------------------------------|----------------------------------|
| North                             |                                  |
| <input type="text" value="50"/>   |                                  |
| West                              | East                             |
| <input type="text" value="-125"/> | <input type="text" value="-65"/> |
| South                             |                                  |
| <input type="text" value="25"/>   |                                  |

**Circle**

Center Latitude

Center Longitude

Inside Radius (km)

Outside Radius (km)

Output Format: CSV

**Advanced Search Options****DEPTH (KM)**

Minimum

Maximum

**AZIMUTHAL GAP**

Minimum

Maximum

**REVIEW STATUS**

- ☒ Any  
☐ Automatic  
☐ Reviewed

**+ EVENT TYPE****+ IMPACT** (PAGER, SHAKEMAP, DYFI)**+ CATALOG****+ CONTRIBUTOR****+ PRODUCT TYPE****Output Options****FORMAT**

- ☐ Map & List  
☒ CSV  
☐ KML  
☐ QuakeML  
☐ GeoJSON

**ORDER BY**

- ☒ Time - Newest First  
☐ Time - Oldest First  
☐ Magnitude - Largest First  
☐ Magnitude - Smallest First

**LIMIT RESULTS**

Number of Events

Offset

Share this page: [Facebook](#) [Twitter](#) [Google](#) [Email](#)
